# Supplementary material for: A New Family of Weighted One-Parameter Flux Reconstruction Schemes
Source: arXiv:1809.07846 source file (2020-06-24)
Supplement: Supplementary file 1 [file appendix_lcl.tex]

%!TEX root = ./gjfr_main.tex
\section{Lumped Chebyshev-Lobatto} \label{app:lcl}
		
	Huynh~\cite{Huynh2007} introduced the concept that correction functions could be 'lumped', this is where the value of the correction function gradient at the solution quadrature points is zeros. This has the benefit of making the correction matrices sparse. A further constraint that he gradient at the opposite flux point was also added to fully constrain the problem and was added as it was believed to increase temporal stability. An important correction function that was introduced was the Lumped-Gauss--Lobatto, which was shown to have very good temporal stability~\cite{Vincent2011} and was found to lie in the OSFR set~\cite{Vincent2010}. However, a Lumped-Cheybshev--Lobatto (LCL) correction was also introduced that was not in the OSFR set, and its inclusion in a correction function set has been elusive, in other than the very general GSFR set. We wish to know if LCL can be included in the GJFR set, which may give some insight into the function behaviour.
	
	We begin by defining the interior points of the Chebyshev-Lobatto quadrature as:		
	\begin{equation}
		\eta_n = \cos{\bigg(\frac{n\pi}{p}\bigg)} \quad \mathrm{for} \quad n\in\{1\dots p-1\}
	\end{equation}
	Hence, the LCL correction function may be defined as:
	\[
	\dx{h_L}{\zeta} = g_L = (1-\zeta)\prod^{p-1}_{n=1}\big[\eta_n - \zeta\big] = (-1)^p(1-\zeta)U_{p-1}(\zeta)
	\]
	The term on the RHS is a Chebyshev polynomial of the second kind, which has the same zeros as the interior points of Chebychev--Lobatto quadrature. Chebyshev polynomials of the second kind are defined by the of three term recurrence relation:
	\begin{equation}
		U_{n+1} = 2xU_n - U_{n-1}, \quad U_0 = 1 \quad\mathrm{and}\quad U_{-1} = 0
	\end{equation}
	This therefore allows the correction function gradient to be written as:
	\[
		g_L = (-1)^p\bigg[U_{p-1} - \half\Big(U_{p} + U_{p-2}\Big)\bigg]
	\]
	Chebyshev polynomials of the second kind can be cast as Jacobi polynomials via:
	\begin{equation}
		U_p(x) = (p+1)\frac{J^{(0.5,0.5)}_p(x)}{J^{(0.5,0.5)}_p(1)} = \frac{(p+1)\Gamma(p+1)\Gamma(1.5)}{\Gamma(p+1.5)}J^{(0.5,0.5)}_p(x)
	\end{equation}
	Hence,
	\begin{equation}
		g_L = (-1)^p\Gamma(1.5)\bigg[\frac{p(p-1)!}{\Gamma(p+0.5)}J^{(0.5,0.5)}_{p-1} - \half\Big(\frac{(p-1)(p-2)!}{\Gamma(p-0.5)}J^{(0.5,0.5)}_{p-2} + \frac{(p+1)p!}{\Gamma(p+1.5)}J^{(0.5,0.5)}_p\Big)\bigg]\label{eq:gl_lcl}
	\end{equation}
	
	To find if this may be included in the set of GJFR correction functions, it will be most straightforward to compare the coefficients of Eq.~(\ref{eq:gl_lcl}) with the gradient of the correction function found earlier. Therefore, we need to differentiate the definition of $h_L$, for which it will be useful to have the identity:		
	\begin{equation}
		\dx{J_p^{(\alpha,\beta)}(x)}{x} = \half(p+\alpha+\beta+1)J_{p-1}^{(\alpha+1,\beta+1)}(x)
	\end{equation}		
	Also for brevity we will define:
	\[
	B^\gamma_p = \frac{(p+1)(p+\gamma)}{\iota p(p+1) + (p+\gamma+1)(p+\gamma)A_p}
	\]	
	and
	\[
	\hat{\alpha} = \alpha + 1
	\]	
	\[
	\hat{\beta} = \beta + 1
	\]	
	Consequently, we may write the derivative of the GJFR correction functions as:
	\begin{subequations}
		\begin{align}
			g_L &= \frac{(-1)^p}{2\kappa_p^{(\alpha,\beta)}}\bigg((p+\alpha+\beta+1)J^{(\hat{\alpha},\hat{\beta})}_{p-1} - B^\alpha_p\bigg[\iota(p+\alpha+\beta)J^{(\hat{\alpha},\hat{\beta})}_{p-2} + (p+\alpha+\beta+2)A_pJ^{(\hat{\alpha},\hat{\beta})}_{p}\bigg] \bigg) \\
			g_R &= \frac{1}{2\kappa_p^{(\beta,\alpha)}}\bigg((p+\alpha+\beta+1)J^{(\hat{\alpha},\hat{\beta})}_{p-1} + B^\beta_p\bigg[\iota(p+\alpha+\beta)J^{(\hat{\alpha},\hat{\beta})}_{p-2} + (p+\alpha+\beta+2)A_pJ^{(\hat{\alpha},\hat{\beta})}_{p}\bigg] \bigg)
		\end{align}
	\end{subequations}
	
	Therefore, to  for the LCL correction function to be in the GJFR set at $\alpha=\beta=-0.5$ an $\iota$ value must exist such that:
	\begin{subequations}
		\begin{align}
			C\frac{\Gamma(1.5)(p-1)(p-2)!}{\Gamma(p-0.5)} &= \frac{\iota(p+\alpha+\beta)B_p^\alpha}{\kappa_p^{(\alpha,\beta)}} \\
			C\frac{\Gamma(1.5)(p+1)p!}{\Gamma(p+1.5)} &= \frac{(p+\alpha+\beta+2)A_pB^\alpha_p}{\kappa^{(\alpha,\beta)}_p}
		\end{align}			
	\end{subequations}
	where $C$ is found by equating the $p-1^\mathrm{th}$ order terms hat are not dependent of $\iota$.
	\[
		C = \frac{(p+\alpha+\beta+1)\Gamma(p+0.5)}{2p(p-1)!\Gamma(1.5)\kappa^{(\alpha,\beta)}_p}
	\]
	There are several ways to solve these equations, the most straightforward is to rearrange each of them for $\iota$. In which case you find that the $\iota$ terms are different and hence LCL is not in GJFR for $\alpha=\beta=-0.5$. Due to the uniqueness of a polynomial based on its zeros, it can therefore be asserted that LCL is not in the GJFR correction function set.
