# Supplementary material for: A New Family of Weighted One-Parameter Flux Reconstruction Schemes
Source: arXiv:1809.07846 source file (2020-06-24)
Supplement: Supplementary file 2 [file appendix_qdg.tex]

%!TEX root = ./gjfr_main.tex
\section{Quasi-DG Schemes}\label{app:qdg}
	In this section we will analyse the qDG schemes that were led out in section~\ref{sec:limits}~\&~\ref{sec:conv}. In particular we wish to understand if this set of schemes corresponds to DG in an alternative basis with respect to weight function. 

	\subsection{Method of Weighted Residuals}	
	Let us begin by setting forth the method of weighted residuals. First we will define the linear advaction equation in the $n^\mathrm{th}$ element as:
	\begin{equation} \label{eq:lin_adv_qdg}
		\px{u_n}{t} + a\px{u_n}{x} = 0 \quad x \in \mathbf{\Omega}_n
	\end{equation}
	where
	\begin{equation}
		u_n = \sum^p_{i=0}\tilde{u}_i\phi_i
	\end{equation}
	for some basis $\phi$. If we now define the residual as:
	\begin{equation}
		R_n = \px{u_n}{t} + a\px{u_n}{x}
	\end{equation}
	A DG solution is then defined by finding a solution $u_n$ such that the residual is orthogonal to the solution basis. 
	\begin{equation}
		\int_{\mathbf{\Omega}_n} R_n \phi_i w(x)\mathrm{d}x = 0
	\end{equation}
	where $w(x)$ is a positive semi-definite weight function. This leads to Eq.~(\ref{eq:lin_adv_qdg}) being written as:
	\begin{equation}
		\int_{\mathbf{\Omega}_n} \phi_i\px{u_n}{t} w(x)\mathrm{d}x + a\int_{\mathbf{\Omega}_n} \phi_i\px{u_n}{x} w(x)\mathrm{d}x = 0
	\end{equation}	
	Applying integration by parts twice to the spatial derivative we obtain:
	\begin{equation}\label{eq:dg}
		\int_{\mathbf{\Omega}_n} \phi_i\px{u_n}{t} w(x)\mathrm{d}x + a\int_{\mathbf{\Omega}_n} \phi_i\px{u_n}{x} w(x)\mathrm{d}x = a\Big|\big(u_n - u^{I}_n\big)\phi_i w(x)\Big|^{x_{n+1}}_{x_n}
	\end{equation}
	This may then be cast in matrix form as:
	\begin{subequations}\label{eq:mat_dg}
		\begin{align}
			\mathbf{M}\dx{\mathbf{u}}{t} + a\mathbf{S}\mathbf{u} &= a\Big|\big(u_n - u^{I}_n\big)w(x)\mathbf{\Phi}(x)\Big|^{x_{n+1}}_{x_n} \\
			\mathbf{M}_{ij} &= \int \phi_i\phi_j w(x) \mathrm{d}x \\
			\mathbf{S}_{ij} &= \int \phi_i\dx{\phi_j}{x} w(x) \mathrm{d}x \\
			\mathbf{\Phi}(x) &= [\phi_0(x), \phi_1(x), \dots ,\phi_p(x)]^T
		\end{align}
	\end{subequations}
	This is the same notation and form that was presented by Karniadakis~\etal~\cite{Karniadakis2013} and Allaneau~\etal~\cite{Allaneau2011}.
	
	\subsection{Weighted Flux Reconstruction}	
	If we now examine the FR scheme that has been defined in this work, let use begin by applying the FR method to Eq.~(\ref{eq:lin_adv_qdg}) as:
	\begin{equation}
		\px{u}{t} + a\px{u}{x} + (f^I_L - f_L)g_L(x) +  (f^I_R - f_R)g_R(x) = 0
	\end{equation}
	Now multiplying by the weight function, $w$, and basis polynomial, then integrating over the sub-domain we reach:
	\begin{multline}
		\int_{\mathbf{\Omega}_n} \phi_i\px{u_n}{t} w(x)\mathrm{d}x + a\int_{\mathbf{\Omega}_n} \phi_i\px{u_n}{x} w(x)\mathrm{d}x + \\
		(f^I_L - f_L)\int_{\mathbf{\Omega}_n} \phi_i g_L(x) w(x)\mathrm{d}x + (f^I_R - f_R)\int_{\mathbf{\Omega}_n} \phi_ig_R(x) w(x)\mathrm{d}x = 0 
	\end{multline}
	applying integration by parts to the final two terms and rearranging, we achieve:
	\begin{multline}
		\int_{\mathbf{\Omega}_n} \phi_i\px{u_n}{t} w(x)\mathrm{d}x + a\int_{\mathbf{\Omega}_n} \phi_i\px{u_n}{x} w(x)\mathrm{d}x =\\
		+ (u_L - u^I_L)\bigg[\big|\phi_iwh_L\big|^1_{-1} - \int_{\mathbf{\Omega}_n} (\phi_iw)^\prime h_L(x) \mathrm{d}x \bigg] \\
		+ (u_R - u^I_R)\bigg[\big|\phi_iwh_R\big|^1_{-1} - \int_{\mathbf{\Omega}_n} (\phi_iw)^\prime h_R(x) \mathrm{d}x \bigg]
	\end{multline}
	This may then be simplified by the boundary conditions on $h_L$ and $h_R$ to:
	\begin{multline}\label{eq:mat_fr}
		\int_{\mathbf{\Omega}_n} \phi_i\px{u_n}{t} w(x)\mathrm{d}x + a\int_{\mathbf{\Omega}_n} \phi_i\px{u_n}{x} w(x)\mathrm{d}x = \Big|\big(u_n - u^{I}_n\big)\phi_i w(x)\Big|^{x_{n+1}}_{x_n} \\
		+ (u^I_L - u_L)\int_{\mathbf{\Omega}_n} (\phi_iw)^\prime h_L(x) \mathrm{d}x + (u^I_R - u_R)\int_{\mathbf{\Omega}_n} (\phi_iw)^\prime h_R(x) \mathrm{d}x 
	\end{multline}
	By comparing this to Eq.~(\ref{eq:dg}), it is clear that if the final two terms on the right-hand side are zero then the schemes are equivalent. Let us begin by expanding the terms $(\phi_iw))^\prime$ as:
	\begin{equation}
		\int_{\mathbf{\Omega}_n} (\phi_iw)^\prime h_L(x) \mathrm{d}x = \int_{\mathbf{\Omega}_n} \phi_i^\prime w h_L(x) \mathrm{d}x + \int_{\mathbf{\Omega}_n} \phi_iw^\prime h_L(x) \mathrm{d}x 
	\end{equation}
	 For the case of Legendre polynomial, when $w(x)=1$, the final term of the right-hand side is zeroed. Then, considering that the basis has a maximum order of $p$, the second can be zeroed by restricting the correction function to the $p^\mathrm{th}$ and $p+1^\mathrm{th}$ order mode as was found by Huynh~\cite{Huynh2007}. To find if the qDG scheme can also lead to equivalence we will brake down these terms further.
	
	For the qDG schemes, when $\iota=0$, we can see from Eq.~(\ref{eq:hl}) that $h_L$ is also restricted to the $p^\mathrm{th}$ and $p+1^\mathrm{th}$ order modes. This leads to the first term on the RHS to be zeros. However, the second term, due to the gradient of the weight function, cannot be straightforwardly set to zero. The Legendre case gives $w^\prime = 0$, but for Jacobi polynomials in general considered differentiating $w$.
	\[
		\dx{w^{(\alpha,\beta)}}{x} = \beta w^{(\alpha,\beta-1)} - \alpha w^{(\alpha-1,\beta)}
	\]   
	Therefore, it is required that when the basis of $h_L$ is changed from $(\alpha,\beta)$ to $(\alpha,\beta-1)$ and $(\alpha-1,\beta)$ it solely has $p+1^\mathrm{th}$ order terms. This is would contradict the boundary condition on $h_L$ and so $\iota=0$ does not lead to FR being equivalent to DG in a different basis. Hence, quasi-DG only symbolises that the norm is analogous to the one case in which equivalence can be found. 
	
	\subsection{GJFR as Filtered DG}
	Through a similar analysis we may inspect if this the GJFR correction functions may be written as linearly filtered DG. We begin by writing Eq.~(\ref{eq:mat_fr}) in matrix similar to Eq.~(\ref{eq:mat_dg}): 
	\begin{multline}
		\mathbf{M}\dx{\mathbf{u}}{t} + a\mathbf{S}\mathbf{u} = \mathbf{RHS}_{DG}
		+ \rint{(u_{CL}h_L + u_{CR}h_R)w\mathbf{\Phi}^\prime}{x} \\
		+ \rint{(u_{CL}h_L + u_{CR}h_R)w^\prime\mathbf{\Phi}}{x}
	\end{multline}
	where $u_{CL} = u_L^I - u_L$ and $\mathbf{RHS}_{DG}$ is the right-hand side term from Eq.~(\ref{eq:dg}).	To proceed we will use the methodology of Allaneau~\etal~\cite{Allaneau2011} by defining a matrix $\mathbf{K}$ such that $\mathbf{KD} = 0$. Where $\mathrm{d}\mathbf{u}/\mathrm{d}x = \mathbf{Du}$. Hence, we can write:
	\begin{equation}
		\mathbf{K}\dx{\mathbf{u}}{t} = -u_{CL}\mathbf{Kh}_L - u_{CR}\mathbf{Kh}_R
	\end{equation}
	Combining these we get:
	\begin{multline}
		(\mathbf{M} + \mathbf{K})\dx{\mathbf{u}}{t} + a\mathbf{Su} = \mathbf{RHS}_{DG} 
		+ u_{CL}\bigg[\rint{h_Lw\mathbf{\Phi}^\prime + h_Lw^\prime\mathbf{\Phi}}{x}  - \mathbf{Kh}_L\bigg] \\
		+ u_{CR}\bigg[\rint{h_Rw\mathbf{\Phi}^\prime + h_Rw^\prime\mathbf{\Phi}}{x}  - \mathbf{Kh}_R\bigg]
	\end{multline}
	which from Eq.~(\ref{eq:hl_cond}-\ref{eq:hr_cond}) can be written as:
	\begin{multline}
		(\mathbf{M} + \mathbf{K})\dx{\mathbf{u}}{t} + a\mathbf{Su} = \mathbf{RHS}_{DG} + u_{CL}\rint{h_Lw^\prime\mathbf{\Phi}}{x} + u_{CR}\rint{h_Rw^\prime\mathbf{\Phi}}{x}
	\end{multline}
	Hence, again due to the derivative of the weight function being non-zero, we can see that GJFR correction function are not equivalent to linearly filtered DG.
%	
%	\subsection{Trying to solve the stability limit}
%		
%		If we define matrices to transform from particular Jacobi bases as:
%		\begin{subequations}
%			\begin{align}
%				\tilde{\mathbf{u}}_{(\alpha,\beta)} &= \mathbf{A}\tilde{\mathbf{u}}_{(\alpha-1,\beta)} \\
%				\tilde{\mathbf{u}}_{(\alpha,\beta)} &= \mathbf{B}\tilde{\mathbf{u}}_{(\alpha,\beta-1)} 
%			\end{align}
%		\end{subequations}
%		
%		therefore the conditions on stability can be framed as:
%		
%		\begin{subequations}
%			\begin{align}
%				&\bigg[\beta{\big(\mathbf{B}^{-1}\big)}^T \mathbf{M}_{(\alpha,\beta-1)}\mathbf{B} - \alpha{\mathbf{A}^{-1}}^T \mathbf{M}_{(\alpha-1,\beta)}\mathbf{A} + \underbrace{\mathbf{D}^T\mathbf{M} - \iota\big(\mathbf{D}^p\big)^T\mathbf{MD}^{p+1}}_{\mathrm{Eq.(30)}}\bigg]\tb{h}_L = 0 \\
%				&h_L(-1) = 0 \\
%				&h_L(1) = 0
%			\end{align}
%		\end{subequations}
%		typically you can insert the boundary conditions as extra lines in matrix on the right hand side of 92a. But in this case the rank of the matrix is p+1 and not p, as is the case in OSFR.
%		
%		We also can't use:
%		\[
%			\int^b_a f(x) g(x) \mathrm{d}x \leqslant \max_{x\in[a,b]}{\big(g(x)\big)}\int^b_a f(x) \mathrm{d}x 
%		\]
%		as this requires both $f$ and $g$ to be positive definite, and although $g$ is we can't make any such statements about $\partial(uh_L)/\partial x$
%	
